# Supplementary material for: Terrestrial campaign towards space-to-ground quantum communications with a space-qualified entangled photon-pair system
Source: arXiv:2605.19689 source file (2026-10-28)
Supplement: Supplementary file 1 [file supplementary.tex]

\documentclass[aps,pra,onecolumn,superscriptaddress, notitlepage,10pts]{revtex4-1}
\usepackage{graphicx} % Required for inserting images
\usepackage{lipsum}
\usepackage{orcidlink}
\usepackage{xcolor}
\usepackage{subcaption}
\usepackage{url}
\usepackage{amsmath}

% \date{November 2025}

\begin{document}

\title{Supplementary Material}

\maketitle

\section{Key-rate analysis}

We summarize the procedure used to estimate the secret key rate for the BBM92 protocol. Two cases are considered: the asymptotic limit and the finite-key analysis using the sharp statistical bound.

\subsection{Preliminaries}

For each data block, we denote:
\begin{itemize}
    \item $N$: total number of sifted pairs,
    \item $n$: number of bits used for parameter estimation,
    \item $n_{\mathrm{key}} = N - n$: number of key-generation bits,
    \item $\hat{p}$: observed quantum bit error rate (QBER),
    \item $\epsilon$: total security parameter.
\end{itemize}

We used $n = 0.20 N$ (20\% for parameter estimation, 80\% for key generation).

The binary entropy function is defined as:
\begin{equation}
h(x) = -x \log_2 x - (1-x)\log_2(1-x),
\end{equation}

The security parameter is divided as:
\begin{equation}
\epsilon = \epsilon_{\mathrm{PE}} + \epsilon_{\mathrm{sec}} + \epsilon_{\mathrm{cor}},
\end{equation}
corresponding to parameter estimation, secrecy, and correctness, respectively. We used an equal splitting $\epsilon_{\mathrm{PE}} = \epsilon_{\mathrm{sec}} = \epsilon_{\mathrm{cor}} = \epsilon / 3$, with a total security parameter of $\epsilon = 4 \times 10^{-16}$.

\subsection{Asymptotic Key Rate}

In the asymptotic limit, the secret key length is given by \cite{ma2007quantum}:
\begin{equation}
S_{\mathrm{asym}} =  \max \left\{ 0,
n_{\mathrm{key}} \left[ 1 - f_{\mathrm{EC}} \, h(\hat{p}) - h(\hat{p}) \right] \right\},
\end{equation}
where $f_{\mathrm{EC}}$ denotes the error correction efficiency. Note that the basis reconciliation factor is equal to one because the rate is calculated using sifted pairs, i.e., after basis reconciliation. 

% \subsection*{C. Finite-Key Rate with Serfling Bound}

% To account for finite-size effects, we first bound the phase error rate using the Serfling inequality \cite{serfling1974probability,islam2024finite}. The statistical fluctuation term is given by:
% \begin{equation}
% \nu = \sqrt{\frac{(N - n + 1)\ln(1/\epsilon_{\mathrm{PE}})}{2 n N}}.
% \end{equation}

% The corresponding upper bound on the phase error rate is:
% \begin{equation}
% \label{threshold_serfling}
% q^{\mathrm{th}}_{\mathrm{Serf}} = \min\left(1, \frac{N(\hat{p} + \nu) - n\hat{p}}{N - n}\right).
% \end{equation}

% The finite-key secret key length is then:
% \begin{equation}
% S_{\mathrm{Serf}} =  \max \left\{ 0, 
% n_{\mathrm{key}} \left[ 1 - h(q^{\mathrm{th}}_{\mathrm{Serf}}) \right]
% - f_{\mathrm{EC}} \,n_{\mathrm{key}} \,h(\hat{p})
% - \Delta\right\},
% \end{equation}

% where the finite-key correction term is:
% \begin{equation}
% \Delta = 6 \log_2\left(\frac{1}{\epsilon_{\mathrm{sec}}}\right)
% + \log_2\left(\frac{2}{\epsilon_{\mathrm{cor}}}\right).
% \end{equation}

\subsection{Finite-Key Rate with Sharp Bound}

We next consider the tighter statistical bound introduced in \cite{mannalath2025sharp}. 

By defining:
\begin{equation}
\kappa_{n,\epsilon} = \frac{2}{9n}\ln\left(\frac{1}{\epsilon_{\mathrm{PE}}}\right),
\end{equation}

the function $\gamma^{+}_{n,\epsilon}(x)$ is given by:
\begin{equation}
\gamma^{+}_{n,\epsilon}(x)
=
\frac{1}{1 + 4\kappa_{n,\epsilon}}
\left[
3\kappa_{n,\epsilon}
+ (1 - 2\kappa_{n,\epsilon})x
+ 3\sqrt{\kappa_{n,\epsilon}(\kappa_{n,\epsilon} + x - x^2)}
\right].
\end{equation}
Note that the bound $\gamma^{+}_{n,\epsilon}(x)$ is valid for $\kappa_{n,\epsilon} \le 1/4$; if this condition is violated due to an exceedingly small sample size $n$, we set $q^{\mathrm{th}}_{\mathrm{Sharp}} = 1$.

The confidence interval is defined piecewise as:
\begin{equation}
\Gamma^{+}_{n,\epsilon}(x) =
    \begin{cases}
    \gamma^{+}_{n,\epsilon}(x)  \quad \text{if } x \in \bigg[0, \frac{1 - 2\kappa_{n,\epsilon}}{1 + \kappa_{n,\epsilon}} \bigg] \\
    1 + \epsilon \quad \text{otherwise}.
    \end{cases}
\end{equation}

Following Proposition 2 of \cite{mannalath2025sharp}, the phase error threshold for the remaining bits is:
\begin{equation}
\label{threshold_sharp}
q^{\mathrm{th}}_{\mathrm{Sharp}} =
\frac{N \, \Gamma^{+}_{n,\epsilon}(\hat{p}) - n \,\hat{p}}{N - n}.
\end{equation}

The phase error threshold in Eq. \ref{threshold_sharp} is bounded to the interval $[0,1]$. The corresponding finite-key secret key length is:

\begin{equation}
S_{\mathrm{Sharp}} = \max \left\{ 0, 
n_{\mathrm{key}} \left[ 1 - h(q^{\mathrm{th}}_{\mathrm{Sharp}}) \right] 
- f_{\mathrm{EC}} \, n_{\mathrm{key}} \,  h(\hat{p}) 
- \Delta \right\}.
\end{equation}

\section{LEO Satellite extrapolation}
In the 1.8~km QKD experiment, a mean sifted coincidence rate of 24665~cps was obtained. We extrapolate this to a LEO link by considering the expected geometric loss in a downlink from SpeQtre to ADQOGS. 

Using the Two-Line Element (TLE) of SpeQtre on 9 April 2026, 18:27, SpeQtre's pass over ADQOGS was calculated over the next seven days. Five of these passes, with varying maximum elevation angles ranging from 32$^\circ$ to 80$^\circ$ (Fig. \ref{fig:elevation_angles}, were analyzed to determine the expected number of sifted coincidence events over each pass.

For each pass, the geometric loss was calculated. An additional 6~dB of loss was added on top of the geometric loss to account for atmospheric attenuation and tracking errors. The number of sifted coincidences collected was integrated over the pass. Finite-key analysis was done to extract the key rate for each pass. The results are tabulated in Table \ref{tbl: pass_keyrates}.

\begin{figure}[h!]
    \centering
    \includegraphics[width=0.7\linewidth]{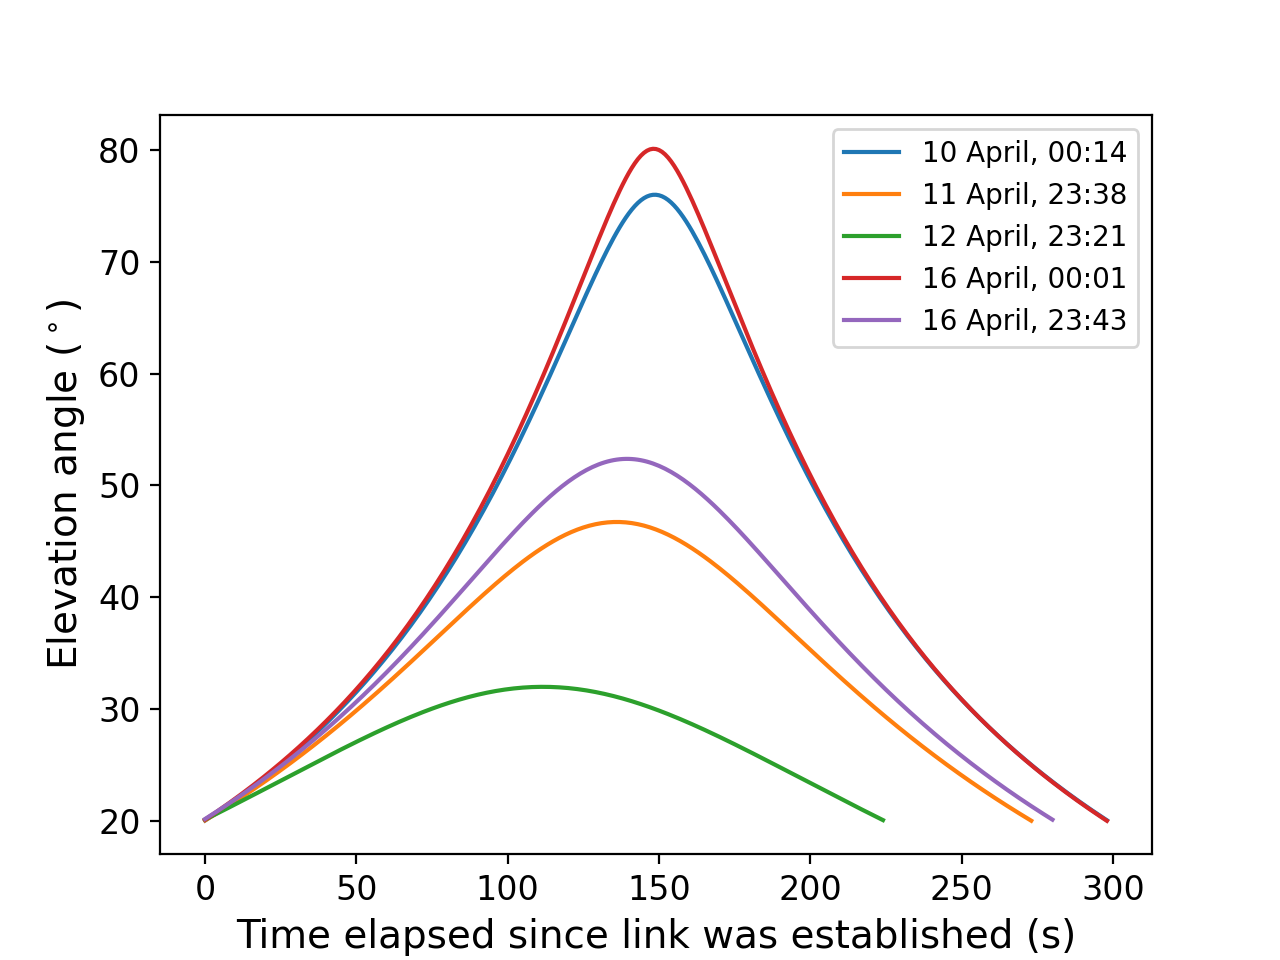}
    \caption{Elevation angles throughout some simulated passes of SpeQtre over ADQOGS, simulated using SpeQtre's TLE from 9 April 2026, 18:27. The labels refer to the local time (UTC+4) when the link is first established. The link remains established when the elevation angle $\geq20^\circ$.}
    \label{fig:elevation_angles}
\end{figure}

\begin{table}[h]
\setlength{\tabcolsep}{15pt}
\centering
\begin{tabular}{ c c c c c }
\hline
Local time of satellite pass  & Maximum elevation angle & Link duration & Secret key rate (bps) \\ \hline
10 April, 00:14 & 76$^\circ$ & 299~s & 4.14  \\ \hline
11 April, 23:38 & 47$^\circ$ & 274~s & 1.45  \\ \hline
12 April, 23:21 & 32$^\circ$ & 225~s & 0  \\ \hline
16 April, 00:01 & 80$^\circ$ & 299~s & 4.31  \\ \hline
16 April, 23:43 & 52$^\circ$ & 281~s & 2.17  \\ \hline
\end{tabular}
\caption{Secret key rates expected for various passes of SpeQtre over ADQOGS.}
\label{tbl: pass_keyrates}
\end{table}

\bibliography{biblio.bib}
\end{document}
